# Supplementary material for: HERGen: Elevating Radiology Report Generation with Longitudinal Data
Source: arXiv:2407.15158 source file (2024-07-21)
Supplement: Supplementary file 1 [file x_supp.tex]

\subsection{Modules}

\para{Image Encoder.}
\label{para:image encoder}
Following the insights from CvT-212DistilGPT2~\cite{nicolson2023improving}, we utilize the CvT architecture~\cite{wu2021cvt}, pretrained on ImageNet-21K, as the foundation for our image encoder. 
This choice is supported by empirical evidence demonstrating its effectiveness in interpreting radiological images.
Subsequently, an encoder projection layer $E_{\mathrm{proj}}$ is integrated to align the number and dimension of visual tokens with the text decoder's needs.

Formally, for each patient, indexed by $i$, our image encoder $E$ processes its series of chest X-rays $\mathcal{I}_i = \{\mathbf{I}_1^{(i)}, \mathbf{I}_2^{(i)}, ..., \mathbf{I}_{N_i}^{(i)}$\} into visual features $\mathcal{P}_i = \{\mathbf{P}_1^{(i)}, \mathbf{P}_2^{(i)}, ..., \mathbf{P}_{N_i}^{(i)}$\}.
Each X-ray image $\mathbf{I}_j^{(i)} \in \mathbb{R}^{C\times W \times H}$ ($0 \leq j \leq N_i-1$), with $C$, $H$, and $W$ representing the number of channels, height, and width respectively, is encoded into a feature representation $\mathbf{P}_j^{(i)}$ in $\mathbb{R}^{S\times F}$.
Here, $S$ and $F$ denote the number of visual tokens and the feature dimension per token, respectively.
To adjust the dimension of visual features and the number of visual tokens, we introduce an encoder projection layer $E_{proj}$, consisting of a $1\times 1$ convolution layer followed by a linear projection layer.
Specifically, $E_{proj}$ transforms each $\mathbf{P}_j$ ($0 \leq j \leq N_i-1$) into a more compact visual representation $\mathbf{V}_j$, resulting in $\mathcal{V}_i = \{\mathbf{V}_1^{(i)}, \mathbf{V}_2^{(i)}, ..., \mathbf{V}_{N_i}^{(i)}\}$ in $\mathbb{R}^{S' \times F'}$, where $S'$ and $F'$ represent the adjusted number of visual tokens and their new dimensionality.
In our experiments, we set $S'=50$ and $F'=768$.

\para{Text Encoder.}
To accurately interpret the specialized language of radiology reports, we incorporates CXR-BERT~\cite{bannur2023learning}, a BERT-based model specifically fine-tuned on a vast collection of radiology texts, as the text encoder of our framework.
This choice enables our model to produce detailed text embeddings that capture the clinical nuances and specific terminologies of radiology, laying a strong foundation for the subsequent stages of report generation.

Formally, for each patient indexed by $i$, the text encoder transforms their series of radiology reports $\mathcal{R}_i = \{\mathbf{R}_1^{(i)}, \mathbf{R}_2^{(i)}, ..., \mathbf{R}_{N_i}^{(i)}\}$ into a corresponding series of global text embeddings $\{\mathbf{E}_1^{(i)}, \mathbf{E}_2^{(i)}, ..., \mathbf{E}_{N_i}^{(i)}\}$, where $\mathbf{E}_j^{(i)} \in \mathbb{R}^{F'}, 0 \leq j \leq N_i - 1$ with $L$ being the number of text tokens in each embedding.
Following ~\cite{chen2020generating}, $L$ is set to $128$.

\para{Text Decoder.}
Our model utilizes DistilGPT2~\cite{sanh2019distilbert}, a streamlined version of the GPT-2 architecture~\cite{radford2019language}, pretrained on the diverse WebText corpus.
This distilled version maintains the essential auto-regressive and self-attention features of GPT-2, crucial for nuanced language modeling and text generation.
We have integrated the DistilGPT2 decoder with a multi-head cross-attention module, as ~\cite{vaswani2017attention}, enabling it to effectively integrate visual context from projected image features with textual input, a key aspect in generating contextually rich radiology reports.
Specifically, the implementation of this encoder-decoder framework leverages the HuggingFace Transformer library\footnote{https://huggingface.co/blog/encoder-decoder}, ensuring robust and advanced architecture for our text generation tasks.

In our model, the text decoder generates a series of radiology reports $\mathcal{R}_i = \{\mathbf{\hat{R}}_1^{(i)}, \mathbf{\hat{R}}_2^{(i)}, ..., \mathbf{\hat{R}}_{N_i}^{(i)}\}$ from the visual embeddings $\mathcal{D}_i = \{\mathbf{\hat{D}}_1^{(i)}, \mathbf{\hat{D}}_2^{(i)}, ..., \mathbf{\hat{D}}_{N_i}^{(i)}\}$ for each patient $i$. 
This process is formally expressed as $\mathbf{\hat{R}}_j^{(i)} = \mathrm{Decoder}(\mathbf{\hat{D}}_j^{(i)})$ for each image $j \ (0 \leq j \leq N_i - 1)$.
Then, a cross entropy loss is optimized to classify each text token into ground truth token.

\begin{table*}
    \centering
    \caption{
    Clinical Efficacy (CE) metrics including macro-averaged metrics over 14 observations (denoted by mac-14) and micro-averaged over 5 observations (denoted by mic-5) on MIMIC-CXR.     
    The \textbf{Best} and \underline{2nd best} results are shown in bold and underline, respectively.
    \textcolor{red}{
    $\dagger$ indicates the results are cited from the original papers. 
    Note that they are not strictly comparable with us.
    For the baselines without $\dagger$, their results are obtained by re-running the publicly released codebase on the same preprocessed dataset as we used.
    }
    }
    \label{tab: ce_mimic}
    \resizebox{0.95\textwidth}{!}{%
    \begin{tabu}{c c c c c c c c}
    \toprule
    Method & Year & $P_{\mathrm{mac}-14}$ & $R_{\mathrm{mac}-14}$ & $F_{\mathrm{mac}-14}$ & $P_{\mathrm{mic}-5}$ & $R_{\mathrm{mic}-5}$ & $F_{\mathrm{mic}-5}$ \\
    \midrule
    $\mathcal{M}^2$Transformer~\cite{cornia2020meshed} & 2019 & $0.239$ & $0.173$ & $0.173$ & $0.443$ & $0.275$ & $0.309$ \\
    R2Gen~\cite{chen2020generating} & 2020 & $0.297$ & $0.189$ & $0.193$ & $0.295$ & $0.590$ & $0.393$ \\
    R2GenCMN~\cite{chen2022cross} & 2021 \\
    $\mathcal{M}^2$TR.PROGRESSIVE~\cite{nooralahzadeh2021progressive} & 2021 \\
    R2Gen+RL~\cite{qin2022reinforced} & 2022 \\
    R2GenCMN+RL~\cite{qin2022reinforced} & 2022 \\
    XProNet~\cite{wang2022cross} & 2022 & $0.419$ & $0.230$ & $0.242$ & $0.596$ & $0.353$ & $0.444$ \\
    CvT-212DistilGPT2~\cite{nicolson2023improving} & 2022 & $0.484$ & $0.429$ & $0.427$ & $0.525$ & $0.567$ & $0.545$ \\
    DCL~\cite{li2023dynamic} & 2023 \\
    \midrule
    \modelname (\textbf{Ours}) & - & $0.510$ & $0.478$ & $0.434$ & $0.519$ & $0.592$ & $0.553$ \\
    \midrule
    \midrule
    \multicolumn{8}{c}{
    \footnotesize{Results below are not strictly comparable. For reference only.}
    } \\
    \midrule
    \rowfont{\color{gray}}
    $\mathrm{Contrastive Attention}^{\dagger}$~\cite{ma2021contrastive} & 2021 & $0.352$ & $0.298$ & $0.303$ & $-$ & $-$ & $-$ \\
    \rowfont{\color{gray}}
    $\mathcal{M}^2\mathrm{Trans \ w/ \ NLL}^{\dagger}$~\cite{miura2020improving} & 2021 & - & - & - & $0.489$ & $0.411$ & $0.447$ \\
    \rowfont{\color{gray}}
    $\mathcal{M}^2\mathrm{Trans \ w/ \ NLL+BS}+\mathrm{f}_{C_E}^{\dagger}$~\cite{miura2020improving} & 2021 & - & - & - & $0.463$ & $0.732$ & $0.567$ \\
    \rowfont{\color{gray}}
    $\mathcal{M}^2\mathrm{Trans \ w/ \ NLL+BS}+\mathrm{f}_{C_{\mathrm{EN}}}^{\dagger}$~\cite{miura2020improving} & 2021 & - & - & - & $0.503$ & $0.651$ & $0.567$ \\
    \rowfont{\color{gray}}
    $\mathrm{RGRG}^{\dagger}$~\cite{tanida2023interactive}& 2023 & $0.461$ & $0.475$ & $0.447$ & $0.491$ & $0.617$ & $0.547$ \\
    \rowfont{\color{gray}}
    $\mathrm{KIUT}^{\dagger}$~\cite{huang2023kiut} & 2023 & $0.371$ & $0.318$ & $0.321$ & $-$ & $-$ & $-$ \\
    \rowfont{\color{gray}}
    $\mathrm{METransformer}^{\dagger}$~\cite{wang2023metransformer} & 2023 & $0.364$ & $0.309$ & $0.311$ & $-$ & $-$ & $-$ \\
    \bottomrule
    \end{tabu}
    }
\end{table*}
